# Supplementary material for: IN-Flow: Instance Normalization Flow for Non-stationary Time Series Forecasting
Source: arXiv:2401.16777 source file (2025-02-06)
Supplement: Supplementary file 1 [file appendix_nonstation.tex]

\begin{table*}[ht]
\centering
\resizebox{0.85\linewidth}{!}{
\begin{threeparttable}
%\fontsize{8.5pt}{9.7}\selectfont
\small
\caption{Overall performance comparisons  Non-stationary Transformers \cite{liu2022NonstatTranformers}, where Transformer, Informer and Autoformer, three backbones are coupled into Non-stationary Transformer/Informer/Autoformer  to compare with IN-Flow.
} \label{table:appendix_nonstation }
\begin{tabular}{c|c|cccc|cccc|cccc} 
\toprule
\multicolumn{2}{c}{Method}& 
\multicolumn{2}{c}{ { \scriptsize NStation-Trans } }&\multicolumn{2}{c|}{\scriptsize IN-Flow-Trans}& 
\multicolumn{2}{c}{\scriptsize NStation-Infor}&\multicolumn{2}{c|}{{ \scriptsize IN-Flow-Infor}}& 
\multicolumn{2}{c}{\scriptsize NStation-Auto}&   \multicolumn{2}{c}{\scriptsize IN-Flow-Auto}\\ 
\cmidrule(r){1-2} \cmidrule(r){3-4} \cmidrule(r){5-6} \cmidrule(r){7-8} \cmidrule(r){9-10} \cmidrule(r){11-12} \cmidrule(r){13-14} 
\multicolumn{2}{c}{Metric}&
MSE& MAE&  MSE& MAE&
MSE& MAE&  MSE& MAE&
MSE& MAE&  MSE& MAE\\
\midrule \midrule
\multirow{4}{*}{ \rotatebox{90}{ETTh1} }
&48&1.387&1.919&\textbf{1.135}&\textbf{1.841}&1.442&2.001&\textbf{1.126}&\textbf{1.909}&1.628&2.196&\textbf{1.219}&\textbf{1.943}\\
&96&1.879&2.279&\textbf{1.225}&\textbf{1.953}&1.366&2.104&\textbf{1.311}&\textbf{2.113}&2.170&2.628&\textbf{1.259}&\textbf{2.012}\\
&168&1.935&2.467&\textbf{1.312}&\textbf{2.059}&\textbf{1.376}&\textbf{2.186}&{1.621}&{2.345}&1.793&2.395&\textbf{1.366}&\textbf{2.135}\\
&336&1.683&2.453&\textbf{1.449}&\textbf{2.242}&\textbf{1.872}&\textbf{2.574}&{2.134}&{2.755}&2.086&2.674&\textbf{1.396}&\textbf{2.229}\\
\midrule
\multirow{4}{*}{ \rotatebox{90}{ETTh2} }
&48&1.677&2.537&\textbf{1.352}&\textbf{2.335}&2.094&2.842&\textbf{1.487}&\textbf{2.457}&1.553&2.507&\textbf{1.427}&\textbf{2.435}\\
&96&2.078&2.968&\textbf{1.734}&\textbf{2.672}&2.065&2.906&\textbf{1.761}&\textbf{2.764}&2.021&2.888&\textbf{1.839}&\textbf{2.746}\\
&168&2.198&3.077&\textbf{1.936}&\textbf{2.892}&2.468&3.226&\textbf{1.958}&\textbf{2.949}&2.007&2.946&\textbf{1.815}&\textbf{2.808}\\
&336&2.983&3.477&\textbf{2.053}&\textbf{2.924}&2.710&3.321&\textbf{2.096}&\textbf{3.006}&2.117&3.062&\textbf{2.068}&\textbf{2.978}\\
\midrule
\multirow{4}{*}{ \rotatebox{90}{ETTm2}}
&48&0.948&1.918&\textbf{0.865}&\textbf{1.851}&0.968&1.900&\textbf{0.944}&\textbf{1.941}&1.093&2.133&\textbf{1.028}&\textbf{2.068}\\
&96&1.227&2.161&\textbf{1.026}&\textbf{2.017}&1.299&2.194&\textbf{1.079}&\textbf{2.092}&1.336&2.337&\textbf{1.171}&\textbf{2.181}\\
&168&1.587&2.497&\textbf{1.291}&\textbf{2.292}&1.697&2.436&\textbf{1.355}&\textbf{2.336}&1.633&2.593&\textbf{1.487}&\textbf{2.481}\\
&336&2.126&2.942&\textbf{1.701}&\textbf{2.666}&1.987&2.798&\textbf{1.971}&\textbf{2.745}&2.166&2.970&\textbf{1.949}&\textbf{2.826}\\
\midrule
\multirow{4}{*}{ \rotatebox{90}{Weather}}
&48&0.551&2.063&\textbf{0.360}&\textbf{1.736}&0.566&1.953&\textbf{0.400}&\textbf{1.764}&0.580&2.205&\textbf{0.421}&\textbf{1.871}\\
&96&0.310&1.641&\textbf{0.259}&\textbf{1.519}&0.256&1.492&\textbf{0.249}&\textbf{1.489}&0.360&1.766&\textbf{0.315}&\textbf{1.715}\\
&168&0.389&1.934&\textbf{0.219}&\textbf{1.439}&0.267&1.446&\textbf{0.217}&\textbf{1.427}&0.533&2.119&\textbf{0.248}&\textbf{1.682}\\
&336&0.323&1.873&\textbf{0.210}&\textbf{1.406}&0.289&1.862&\textbf{0.249}&\textbf{1.655}&0.375&2.055&\textbf{0.261}&\textbf{1.723}\\
\midrule
\multirow{4}{*}{ \rotatebox{90}{CAISO}}
&48&0.850&0.463&\textbf{0.757}&\textbf{0.415}&0.861&0.472&\textbf{0.768}&\textbf{0.436}&0.844&0.461&\textbf{0.794}&\textbf{0.463}\\
&96&1.483&0.582&\textbf{0.970}&\textbf{0.466}&1.336&0.561&\textbf{1.026}&\textbf{0.508}&1.285&0.545&\textbf{1.278}&\textbf{0.572}\\
&168&1.799&0.653&\textbf{1.245}&\textbf{0.535}&1.406&0.570&\textbf{1.358}&\textbf{0.570}&1.534&0.619&\textbf{1.331}&\textbf{0.571}\\
&336&2.282&0.766&\textbf{1.548}&\textbf{0.617}&1.805&0.694&\textbf{1.739}&\textbf{0.668}&1.923&0.724&\textbf{1.535}&\textbf{0.659}\\
\midrule
\multirow{4}{*}{ \rotatebox{90}{NordPool}}
&48&1.914&0.792&\textbf{1.269}&\textbf{0.676}&1.761&0.765&\textbf{1.350}&\textbf{0.698}&1.499&0.753&\textbf{1.489}&\textbf{0.736}\\
&96&2.613&0.934&\textbf{1.655}&\textbf{0.787}&2.341&0.913&\textbf{2.013}&\textbf{0.854}&2.096&0.866&\textbf{2.070}&\textbf{0.849}\\
&168&2.834&1.182&\textbf{2.129}&\textbf{0.895}&2.753&1.001&\textbf{2.400}&\textbf{0.934}&2.557&0.966&\textbf{2.429}&\textbf{0.951}\\
&336&2.934&1.110&\textbf{2.785}&\textbf{1.009}&2.591&0.988&\textbf{2.278}&\textbf{0.924}&2.178&0.925&\textbf{2.083}&\textbf{0.891}\\

\midrule
\bottomrule
\end{tabular}
% \begin{tablenotes}
% \item $*$ means N-BEATS is re-implemented for multivariate time series forecasting; see Appendix A.4 for more details.
% \end{tablenotes}
\end{threeparttable}
}
\end{table*}
