# Supplementary material for: IN-Flow: Instance Normalization Flow for Non-stationary Time Series Forecasting
Source: arXiv:2401.16777 source file (2025-02-06)
Supplement: Supplementary file 5 [file appendix_ablation_autoformer.tex]

\begin{table*}[!h]
\centering
\begin{threeparttable}
%\fontsize{8.5pt}{9.7}\selectfont
\small
\caption{Ablation studies when taking Autoformer as the backbone.
} \label{table:appendix_ablation_autoformer}
\begin{tabular}{c|c|cccccccccc}
\toprule
\multicolumn{2}{c}{Method}& 
\multicolumn{2}{c}{ RealNVP }&\multicolumn{2}{c}{ RealNVP-c}& 
\multicolumn{2}{c}{ IN-Flow-J}&\multicolumn{2}{c}{ IN-Flow-T}& 
\multicolumn{2}{c}{IN-Flow}\\ 
\cmidrule(r){1-2} \cmidrule(r){3-4} \cmidrule(r){5-6} \cmidrule(r){7-8} \cmidrule(r){9-10} \cmidrule(r){11-12} 
\multicolumn{2}{c}{Metric}&
MSE& MAE&  MSE& MAE&
MSE& MAE&  MSE& MAE&
MSE& MAE\\
\midrule \midrule

\multirow{4}{*}{ \rotatebox{90}{ETTh2} }
&48&11.276&8.563&1.458&2.497&1.562&2.495&1.531&2.476&\textbf{1.451}&\textbf{2.426}\\
&96&10.591&8.725&2.003&2.917&1.916&2.808&1.889&2.777&\textbf{1.866}&\textbf{2.744}\\
&168&12.026&8.822&2.214&3.151&1.839&2.859&1.826&2.799&\textbf{1.816}&\textbf{2.825}\\
&336&9.636&7.123&3.041&3.680&2.065&3.028&\textbf{2.010}&\textbf{2.965}&{2.061}&{2.980}\\
\midrule
\multirow{4}{*}{ \rotatebox{90}{ETTm2}}
&48&19.477&11.305&1.138&2.198&1.085&2.129&1.044&2.078&\textbf{1.026}&\textbf{2.057}\\
&96&15.140&9.770&1.387&2.398&1.262&2.295&1.236&2.253&\textbf{1.162}&\textbf{2.178}\\
&168&20.759&11.278&1.697&2.640&1.550&2.502&1.478&\textbf{2.458}&\textbf{1.466}&{2.487}\\
&336&24.613&13.106&2.352&3.088&2.706&3.143&1.973&2.839&\textbf{1.966}&\textbf{2.836}\\
\midrule
\multirow{4}{*}{ \rotatebox{90}{Weather}}
&48&1.743&6.973&1.058&5.243&0.465&2.028&\textbf{0.402}&\textbf{1.815}&{0.405}&{1.859}\\
&96&1.466&6.771&0.664&4.238&0.308&1.766&0.328&1.833&\textbf{0.291}&\textbf{1.669}\\
&168&1.410&6.476&0.461&3.406&\textbf{0.254}&\textbf{1.649}&0.306&1.822&{0.259}&{1.721}\\
&336&1.364&6.545&0.422&3.013&0.284&1.853&\textbf{0.242}&\textbf{1.668}&{0.256}&{1.713}\\
\midrule
\multirow{4}{*}{ \rotatebox{90}{CAISO}}
&48&4.751&1.421&1.577&{0.707}&\textbf{0.759}&\textbf{0.443}&0.938&0.504&0.829&0.469\\
&96&6.798&1.635&2.690&0.932&\textbf{1.196}&\textbf{0.549}&1.322&0.583&1.275&0.573\\
&168&6.058&1.527&2.903&0.934&1.478&0.603&1.363&0.590&\textbf{1.308}&\textbf{0.569}\\
&336&5.073&1.350&3.246&1.009&2.075&0.739&\textbf{1.607}&\textbf{0.644}&1.810&0.684\\
\midrule
\multirow{4}{*}{ \rotatebox{90}{NordPool}}
&48&2.469&1.057&1.697&0.812&1.505&0.733&1.564&0.745&\textbf{1.478}&\textbf{0.732}\\
&96&2.207&1.011&2.167&0.896&2.260&0.896&2.104&0.865&\textbf{2.078}&\textbf{0.860}\\
&168&2.815&1.100&2.523&0.973&\textbf{2.329}&\textbf{0.944}&2.628&0.978&2.460&0.962\\
&336&2.570&1.048&2.175&0.920&2.488&0.969&2.163&0.921&\textbf{2.082}&\textbf{0.896}\\
\midrule
\bottomrule
\end{tabular}
\end{threeparttable}
\end{table*}
