# Supplementary material for: IN-Flow: Instance Normalization Flow for Non-stationary Time Series Forecasting
Source: arXiv:2401.16777 source file (2025-02-06)
Supplement: Supplementary file 6 [file appendix_ablation_nbeats.tex]

\begin{table*}[h]
\centering
\begin{threeparttable}
\small
\caption{Ablation studies when taking N-BEATS as the backbone.
} \label{table:appendix_ablation_nbeats}
\begin{tabular}{c|c|cccccccccc}
\toprule
\multicolumn{2}{c}{Method}& 
\multicolumn{2}{c}{ RealNVP }&\multicolumn{2}{c}{ RealNVP-c}& 
\multicolumn{2}{c}{ IN-Flow-J}&\multicolumn{2}{c}{ IN-Flow-T}& 
\multicolumn{2}{c}{IN-Flow}\\ 
\cmidrule(r){1-2} \cmidrule(r){3-4} \cmidrule(r){5-6} \cmidrule(r){7-8} \cmidrule(r){9-10} \cmidrule(r){11-12} 
\multicolumn{2}{c}{Metric}&
MSE& MAE&  MSE& MAE&
MSE& MAE&  MSE& MAE&
MSE& MAE\\
\midrule \midrule

\multirow{4}{*}{ \rotatebox{90}{ETTh2} }
&48&13.823&9.810&1.380&2.422&1.264&2.220&1.240&2.202&\textbf{1.229}&\textbf{2.182}\\
&96&15.647&10.350&1.879&2.842&1.533&2.487&\textbf{1.530}&\textbf{2.479}&1.570&2.496\\
&168&13.493&9.527&2.192&3.083&1.848&2.719&1.772&2.711&\textbf{1.752}&\textbf{2.681}\\
&336&11.690&8.658&2.317&3.335&\textbf{1.872}&\textbf{2.834}&1.961&2.881&1.928&2.847\\
\midrule
\multirow{4}{*}{ \rotatebox{90}{ETTm2}}
&48&12.291&8.917&1.031&2.063&\textbf{0.876}&\textbf{1.847}&0.938&1.925&0.894&1.866\\
&96&12.977&9.053&1.175&2.188&\textbf{0.971}&\textbf{1.918}&0.993&1.933&0.980&1.945\\
&168&14.474&9.799&1.530&2.467&1.231&2.189&{1.214}&2.164&\textbf{1.212}&\textbf{2.162}\\
&336&16.525&10.893&1.826&2.744&1.546&2.479&1.567&2.502&\textbf{1.541}&\textbf{2.477}\\
\midrule
\multirow{4}{*}{ \rotatebox{90}{Weather}}
&48&1.039&4.973&0.533&2.665&0.495&1.840&0.460&1.731&\textbf{0.432}&\textbf{1.698}\\
&96&1.033&5.354&0.225&1.698&0.234&1.365&0.251&1.376&\textbf{0.223}&\textbf{1.328}\\
&168&0.771&4.724&0.183&1.494&0.186&1.303&0.191&1.243&\textbf{0.182}&\textbf{1.217}\\
&336&0.604&4.647&0.190&1.579&0.183&1.416&0.193&1.382&\textbf{0.179}&\textbf{1.311}\\
\midrule
\multirow{4}{*}{ \rotatebox{90}{CAISO}}
&48&4.355&1.412&0.568&0.368&0.541&0.350&0.516&0.345&\textbf{0.514}&\textbf{0.341}\\
&96&5.311&1.530&0.885&0.441&\textbf{0.777}&\textbf{0.419}&0.906&0.434&0.878&0.428\\
&168&5.013&1.495&1.126&0.502&\textbf{1.054}&\textbf{0.481}&1.153&0.494&1.150&0.498\\
&336&3.710&1.213&1.479&0.592&\textbf{1.358}&\textbf{0.571}&1.535&0.607&1.518&0.602\\
\midrule
\multirow{4}{*}{ \rotatebox{90}{NordPool}}
&48&3.137&1.147&1.166&0.643&\textbf{1.137}&\textbf{0.628}&1.188&0.639&1.150&0.632\\
&96&2.541&1.029&1.602&0.758&1.620&0.759&1.597&0.757&\textbf{1.596}&\textbf{0.756}\\
&168&2.008&0.910&2.006&0.870&1.980&0.845&1.972&0.849&\textbf{1.918}&\textbf{0.836}\\
&336&2.100&0.921&2.283&0.927&\textbf{2.052}&\textbf{0.878}&2.082&0.880&2.098&0.884\\
\midrule
\bottomrule
\end{tabular}
% \begin{tablenotes}
% \end{tablenotes}
\end{threeparttable}
\vspace{-0mm}
\end{table*}
